# Supplementary material for: ACoRe: Automated Goal-Conflict Resolution
Source: arXiv:2303.05213 source file (2023-03-09)
Supplement: Supplementary file 1 [file appendix.tex]

\begin{subappendices}
\section{Evolutionary Operators}
\subsubsection{Mutation}
New individuals are generated through the application of the mutation functions $mutate$ described in Definition~\ref{def:ltl-mutation}. 
Given a candidate individual $cR' = (Dom, G')$, the \emph{mutation} operator selects a goal $g' \in G'$ to mutate, leading to a new goal $g''$,  and produces a new candidate specification $cR'' = (Dom, G'')$, where $G''= G' [g' \mapsto g'']$ (i.e., $G''$ looks exactly as $G'$ but goal $g'$ is replaced by the mutated goal $g''$). 
For instance, Figure~\ref{fig:mutants} shows 5 possible mutations that can be generated for formula $\F (p \Implies \G r)$. 
Mutant M1 replaces $\F$ by $\G$, leading to $M1:\G (p \Implies \G r)$.
Mutant $M2:\F (p \land \G r)$ replaces $\Implies$ by $\land$. 
Mutant $M3:\F (p \Implies \neg r)$ replaces $\G$ by $\neg$.
Mutant $M4: \F (true \Implies \G r)$, reduces to $\F \G r$,  replaces $p$ by $\True$, while mutant $M5 : \F (p \Implies \G q)$ replaces $r$ by $q$.

\begin{definition}[LTL Mutation]
\label{def:ltl-mutation}
Given an LTL formula $\phi$, the function $mutate(\phi)$ $= \phi'$ mutates $\phi$ by performing a syntactic modification driven by its syntax. 
Thus, $mutate(\phi) = \phi'$ is inductively defined as follows: 

{\fontsizeformula
\noindent
\textbf{Base Cases:}
\begin{enumerate}
\item if $\phi = \True$, then $\phi' = \False$; otherwise, $\phi' = \True$.
\item if $\phi = p$, then $\phi' = q$, where $p, q \in AP \land p \neq q$.
\end{enumerate}
\noindent
\textbf{Inductive Cases:}
\begin{enumerate}  \setcounter{enumi}{2}
\item if $\phi = o_{1}\phi_1$, where $o_{1} \in \lbrace \neg, \X, \F, \G \rbrace$, then:
\begin{enumerate}
	\item $\phi' = o_{1}' \phi_1$, s.t. $o_{1}' \in \lbrace \neg, \X, \F, \G \rbrace$ and $o_1 \neq o_1'$.
	\item $\phi' = \phi_1$.
	\item $\phi' = o_{1} mutate(\phi_1)$.
	\item $\phi' = q\ o_{2}'\ \phi$, where $q \in AP$ and $o_{2}' \in \lbrace \U, \W, \land, \lor \rbrace$ 
\end{enumerate}
\item if $\phi = \phi_1 o_{2} \phi_2$, where $o_{2} \in \lbrace \vee, \wedge, \U, \R, \W\rbrace$, then:
\begin{enumerate}
    \item $\phi' = \phi_1\ o_{2}'\ \phi_2$, where $o_{2}' \in \lbrace \vee, \wedge, \U, \R, \W\rbrace$ and $o_2 \neq o_2'$.
    \item $\phi' = \phi_{i}$, s.t. $\phi_{i} \in \lbrace \phi_1, \phi_2 \rbrace$ 
    \item $\phi' = mutate(\phi_1)\ o_{2}\ \phi_2$.
    \item $\phi' = \phi_1\ o_{2}\ mutate(\phi_2)$.
\end{enumerate}
\end{enumerate}
\noindent
\textbf{General Cases:}
\begin{enumerate}\setcounter{enumi}{4}
\item $\phi' = o_{1} \phi$ where $o_{1} \in \lbrace \G, \F, \X, \neg \rbrace$.
\item $\phi' = x$, where $x \in \{\True,\False\}\cup AP$
\end{enumerate}
}
\end{definition}
Base cases 1 and 2 replace constants and propositions with other constants or propositions, respectively. 
Inductive case 3 mutates unary expressions: it can change the unary operator by other (3.a), remove the operator (3.b), mutate the sub-expression (3.b), or augment the current formula by including a binary operator and a proposition (3.d). 
Inductive case 4 mutates binary expressions: it can change the binary operator (4.a), remove one of the expressions and the operator (4.b), or mutate one of the sub-expressions (4.c and 4.d).
Cases 5 and 6 are more general \blue{insofar as} the entire formula $\phi$ is augmented with one unary operator (5) or replaced by a constant or proposition (6).
\iffalse
Precisely, given the set of goals $G'=\{G_1', \ldots,G_{i-1}',G_i',G_{i+1}',\ldots G'_m\}$ from individual $cR$, {\OurTool} invokes function  $mutate(G_i') = G_i''$  to produce a  syntactic modification to goal $G_i'$, leading us to the mutated goal $G_i''$.  
Thus, {\OurTool} creates a new individual $cR'' = (Dom, G'')$, where 
$G''=\{G_1', \ldots,G_{i-1}',G_i'',G_{i+1}',\ldots G'_m\}$. 
\fi

\blue{The offspring} will later be assessed by the fitness function of the corresponding search algorithm to analyze how fit it is to resolve the given goal-conflicts. \blue{The four algorithms apply the mutation operators.}

\subsubsection{Crossover}
\red{In the terms of our work, the application of the crossover operators \blue{is} performed by the genetic algorithms (WBGA~\cite{DBLP:books/mit/H1992} and NSGA-III~\cite{DebJain2014}). A crossover operator is regularly combined with a mutation operator during the evolutionary search process, while the main concern is to combine LTL goals from different candidates to generate offspring. The combination function $combine$ is described in Definition~\ref{def:ltl-crossover}. }
%Besides of the mutation operators, they also consider the combination
%The two variants of genetic algorithms that {\OurTool} integrates, i.e.,  WBGA~\cite{DBLP:books/mit/H1992} and  NSGA-III~\cite{DebJain2014}, besides of the mutation operator, they also consider a crossover operator to combine LTL goals from different candidates. To do so, they employ the $combine$ function described in Definition~\ref{def:ltl-crossover}.

\begin{definition}[LTL Combination]
\label{def:ltl-crossover}
Let $\phi$ and $\psi$ be two LTL formulas. Function $combine(\phi,\psi) $ produces a new formula $\phi'$ by performing the following steps:
\begin{enumerate}
    \item It selects a sub-formula $\alpha$ from $\phi$; to be combined;
    \item it selects sub-formula $\beta$ from $\psi$;
    \item it either, (a) $\phi'= \phi[\alpha \mapsto \beta]$ replaces $\alpha$ by $\beta$ in $\phi$; or (b) $\phi'= \phi[\alpha \mapsto \alpha\ o_2\ \beta]$ combines $\alpha$ and $\beta$ with a binary operator $o_{2} \in \lbrace \vee, \wedge, \U, \R, \W\rbrace$.
\end{enumerate}
\end{definition}

\iffalse
\red{Overall,} given two individuals $cR^1 = (Dom, G^1)$ and $cR^2 = (Dom, G^2)$, 
%{\OurTool} 
the crossover applicant selects two goals such that $G_i^1 \in G^1$ and $G_j^2 \in G^2$, and then combines them to produce a new candidate repair $cR'' = (Dom, G'')$. 
Assuming that $G^1=\{G_1^1, \ldots,G_{i-1}^1,G_i^1,G_{i+1}^1,\ldots G^1_m\}$ and $G^2=\{G_1^2, \ldots,G_{j-1}^2,G_j^2,G_{j+1}^2,\ldots G^2_k\}$,
then $G''=\{G_1^1, \ldots,G_{i-1}^1,G_i'',G_{i+1}^1,\ldots G^1_m\}$ where $G_i'' = combine(G_{i}^1,G_j^2)$. 
\fi
\iffalse
\red{To realize the operation, the genetic algorithms employ the $combine$ function described in Definition~\ref{def:ltl-crossover}.}
\fi
\end{subappendices}
